# Supplementary material for: A Riemannian Generalization of Wilks' Lambda for Testing Differences Among Brain Connectomes
Source: arXiv:2511.09431 source file (2026-11-21)
Supplement: Supplementary file 1 [file supplement.tex]

\documentclass{article}

\usepackage{amsmath,amssymb,amsthm}
\usepackage{natbib}
\usepackage{algorithm}
\usepackage{algorithmic}

% Theorem environments

\theoremstyle{definition}

\theoremstyle{remark}

% Custom commands (same as main paper)

% Additional command for norm notation

\title{Supplemental Materials for:\\
A Novel Testing Approach for Differences Among Brain Connectomes}

\author{Nicolas Escobar$^1$ and Jaroslaw Harezlak$^2$\\
$^1$Department of Statistics, Indiana University\\
$^2$Department of Epidemiology and Biostatistics, Indiana University}

\date{}

\begin{document}

\maketitle

\section*{Introduction}

This supplement provides technical details and proofs that support the main paper.
Section 1 contains additional proofs and technical lemmas.
Section 2 provides the necessary background on Riemannian geometry on the manifold of symmetric positive definite matrices.

\section{Technical Details and Additional Proofs}
\label{sec:proofs}

\input{apendice1}

\section{Riemannian Geometry Background}
\label{sec:riemannian}

\input{apendice2}

\end{document}
